# Supplementary material for: LLaVA-NeXT-Interleave: Tackling Multi-image, Video, and 3D in Large Multimodal Models
Source: arXiv:2407.07895 source file (2024-07-28)
Supplement: Supplementary file 1 [file appendix.tex]

\section{Appendix}

\begin{table*}[!ht]
    \centering
    \begin{tabular}{llll}
    \toprule
        Task & Dataset & Scenario & \# Samples \\ \midrule
        \textbf{Multi-image Scenarios} & ~ & ~ & ~ \\ \hline
        Spot the Difference(63.9K) & Real-world Difference & Realistic & 7.5K \\ 
        ~ & Synthetic Difference & Synthetic & 7.5K \\ 
        ~ & COCO Difference & Realistic & 20K \\ 
        ~ & Spot-the-Diff & Surveilance & 11K \\ 
        ~ & Birds-to-Words & Birds & 14K \\ 
        ~ & CLEVR-Change & Solids & 3.9K \\ \hline
        Image Edit Instruction(67.7K) & HQ-Edit & Sythentic & 50K \\ 
        ~ & MagicBrush & Realistic & 14.2K \\ 
        ~ & IEdit & Realistic & 3.5K \\ \hline
        Visual Story Telling(66.9K) & AESOP & Cartoon & 6.9K \\ 
        ~ & FlintstonesSV & Cartoon & 22K \\ 
        ~ & PororoSV & Cartoon & 12K \\ 
        ~ & VIST & Realistic & 26K \\ \hline
        Visual Cloze(14.6K) & COMICS\_Dialogue & Cartoon & 5.9K \\ 
        ~ & RecipeQA\_VisualCloze & Realistic & 8.7K \\ \hline
        Text-rich VQA(21.4K) & WebQA & Webpage & 9.3K \\ 
        ~ & TQA & Textbook & 8.3K \\ 
        ~ & OCR-VQA & OCR & 1.9K \\ 
        ~ & DocVQA & Document & 1.9K \\ \hline
        Multi-image VQA(174.5K) & NLVR2 & Realistic & 83K \\ 
        ~ & MIT-States\_StateCoherence & General & 1.9K \\ 
        ~ & MIT-States\_PropertyCoherence & General & 1.9K \\ 
        ~ & RecipeQA\_ImageCoherence & Recipe & 8.7K \\ 
        ~ & VISION & Industrial & 10K \\ 
        ~ & Multi-VQA & General & 5K \\ 
        ~ & IconQA & General & 64K \\ \hline
        Low-level Comparison(66K) & Coinstruct & Low-level & 50K \\ 
        ~ & Dreamsim & Low-level & 16K \\ \hline
        Image-caption Comprehension (73K) & ImageCoDe & General & 17K \\ 
        ~ & Contrast-Caption & General & 36K \\ 
        ~ & Multi-image Caption & General & 10K \\ \hline
        Daily Scenarios (11K) & MMChat\_Twitter\_Post & General & 10K \\ 
        ~ & Interleaved Multi-image Dialogue & General & 1K \\ \midrule
        Multi-image Puzzle (35K) & Raven & Abstract & 35K \\ \hline
        \textbf{Multi-frame (Video) Scenarios} & ~ & ~ & ~ \\ \hline
        Video QA(247K) & NExT-QA & General & 4K \\ 
        ~ & STAR & General & 3K \\ 
        ~ & ShareGPTVideo-VQA & General & 240K \\ \hline
        Video Detailed Captioning (15K) & ShareGPTVideo-Caption & General & 15K \\ \midrule
        \textbf{Multi-view (3D) Scenarios} & ~ & ~ & ~ \\ \hline
        Scene VQA(45K) & Nuscenes & Outdoor & 10K \\ 
        ~ & ScanQA & Indoor Realistic & 25k \\ 
        ~ & 3D-LLM-Scene & Indoor Realistic & 10K \\ \hline
        Embodied VQA(61K) & ALFRED & Indoor Synthetic & 23K \\ 
        ~ & 3D-LLM-Dialogue & Indoor Realistic & 20K \\ 
        ~ & 3D-LLM-Planning & Indoor Realistic & 18K \\ \hline
        \textbf{Single-image Scenarios} & ~ & ~ & ~ \\ \hline
        Single-image Tasks(307K) & Randomly sampling 40\% SFT data of LLaVA-NeXT & General & 307K \\ \bottomrule
    \end{tabular}
    \caption{M4-Instruct  detailed datasets.}
    \label{tab:m4_instruct_details}
\end{table*}
